# Supplementary material for: Vulnerability-Aware Poisoning Mechanism for Online RL with Unknown Dynamics
Source: arXiv:2009.00774 source file (2022-02-15)
Supplement: Supplementary file 1 [file prelim.tex]

\section{Notations and Preliminaries}\label{app:prelim}

In RL, an agent interacts with the environment by taking actions, observing states and receiving rewards.
The environment is modeled by a Markov Decision Process (MDP), which is denoted by a tuple $\mdp=\langle \states, \actions, \dynamics, \rewards, \gamma \rangle$, where $\states$ is the state space, $\actions$ the action space, $\dynamics$ the transition kernel, $\rewards$ the reward function, and $\gamma \in (0, 1)$ the discount factor.

At every step, the agent selects an action based on the current \textit{policy} $\pi$. A stochastic \textit{policy} $\pi: \states \times \actions \to [0,1]$ defines the probability of choosing each action in each state. 
A trajectory $\tau$ generated by $\pi$ is a sequence $s_1, a_1, r_1, s_2, a_2, \cdots$, where $s_0 \sim \mu$, $a_t \sim \pi(a|s_t)$, $s_{t+1} \sim P(s| s_t, a_t)$ and $r_t = R(s_t, a_t)$.
Define an \textit{observation} sequence as the concatenation of multiple trajectories generated by taking a policy in an environment, denoted as $\obs = (\boldsymbol{s}, \boldsymbol{a}, \boldsymbol{r}, \boldsymbol{d})$, where $\boldsymbol{s}=[s_1,s_2,\cdots], \boldsymbol{a}=[a_1,a_2,\cdots], \boldsymbol{r}=[r_1,r_2,\cdots], \boldsymbol{d}=[d_1,d_2,\cdots]$ are respectively the sequence of states, actions, rewards and the terminal state flags.

The goal of an RL agent is to find a policy $\pi^*$ that maximizes the expected total rewards $\etr$, which is defined as $\etr(\pi) = \mathbb{E}_{\tau \sim \pi}[r(\tau)] = \mathbb{E}_{s_1,a_1,\cdots}[\sum_{t=1}^{\infty} \gamma^{t-1} r_t]$.

The state value function $V^\pi(s)$ is defined as
$V^\pi(s) = \mathbb{E}_{a_t,\cdots}[\sum_{h=0}^{\infty} \gamma^{h} r_{t+h} | s_t=s]$.
Similarly, the state-action value function $Q^\pi(s,a)$ is 
$Q^\pi(s, a) = \mathbb{E}_{s_{t+1},\cdots}[\sum_{h=0}^{\infty} \gamma^{h} r_{t+h} | s_t=s, a_t=a]$
