# Supplementary material for: Vulnerability-Aware Poisoning Mechanism for Online RL with Unknown Dynamics
Source: arXiv:2009.00774 source file (2022-02-15)
Supplement: Supplementary file 2 [file fig_disc_add.tex]

%!TEX root = ../0_neurips2020_poisonrl_main.tex
% \vspace*{-0.5em}
\begin{figure}[!h]
\centering
	\begin{subfigure}[t]{0.24\columnwidth}
		\centering
		\input{\fighome/disc_plots_app/hopper_vpg.tex}
	% \caption{VPG on CartPole}
	% \label{sfig:vpg_cart}
	\end{subfigure}
	\hfill
	\begin{subfigure}[t]{0.24\columnwidth}
		\centering
		\input{\fighome/disc_plots_app/halfc_vpg.tex}
	% \caption{VPG on CartPole}
	% \label{sfig:vpg_cart}
	\end{subfigure}
	\hfill
	\begin{subfigure}[t]{0.24\columnwidth}
		\centering
		\input{\fighome/disc_plots_app/hopper_ppo.tex}
	% \caption{VPG on CartPole}
	% \label{sfig:vpg_cart}
	\end{subfigure}
	\hfill
	\begin{subfigure}[t]{0.24\columnwidth}
		\centering
		\input{\fighome/disc_plots_app/halfc_ppo.tex}
	% \caption{VPG on CartPole}
	% \label{sfig:vpg_cart}
	\end{subfigure}
\vspace{-1.5em}
\caption{\small{Additional results for comparison of policy discrepancies at every iteration. }}
\label{fig:disc_add}
\end{figure}
% \vspace*{-0.5em}
