# Supplementary material for: Vulnerability-Aware Poisoning Mechanism for Online RL with Unknown Dynamics
Source: arXiv:2009.00774 source file (2022-02-15)
Supplement: Supplementary file 3 [file fig_poison_add.tex]

%!TEX root = ../0_neurips2020_poisonrl_main.tex
% \vspace*{-0.5em}
\begin{figure}[!htbp]
\centering
	\begin{subfigure}[t]{0.24\columnwidth}
		\centering
		\input{\fighome/vpg_ppo_app/Hopper_vpg_e=4.0_smooth.tex}
	% \caption{VPG on CartPole}
	% \label{sfig:vpg_cart}
	\end{subfigure}
	\hfill
	\begin{subfigure}[t]{0.24\columnwidth}
		\centering
		\input{\fighome/vpg_ppo_app/HalfCheetah_vpg_e=4.0.tex}
	% \caption{VPG on CartPole}
	% \label{sfig:vpg_cart}
	\end{subfigure}
	\hfill
	\begin{subfigure}[t]{0.24\columnwidth}
		\centering
		\input{\fighome/vpg_ppo_app/CartPole_ppo_e=4.0.tex}
	% \caption{VPG on CartPole}
	% \label{sfig:vpg_cart}
	\end{subfigure}
	\hfill
	\begin{subfigure}[t]{0.24\columnwidth}
		\centering
		\input{\fighome/vpg_ppo_app/HalfCheetah_ppo_e=1.0.tex}
	% \caption{VPG on CartPole}
	% \label{sfig:vpg_cart}
	\end{subfigure}
	\vspace*{-1em}
	\begin{subfigure}[t]{0.24\columnwidth}
		\centering
		\input{\fighome/a2c_acktr_app/Hopper_a2c_e=1.0.tex}
	% \caption{VPG on CartPole}
	% \label{sfig:vpg_cart}
	\end{subfigure}
	\hfill
	\begin{subfigure}[t]{0.24\columnwidth}
		\centering
		\input{\fighome/a2c_acktr_app/Walker2d-v2_a2c_e=1.0.tex}
	% \caption{VPG on CartPole}
	% \label{sfig:vpg_cart}
	\end{subfigure}
	\hfill
	\begin{subfigure}[t]{0.24\columnwidth}
		\centering
		\input{\fighome/a2c_acktr_app/CartPole-v0_acktr_e=2.0.tex}
	% \caption{VPG on CartPole}
	% \label{sfig:vpg_cart}
	\end{subfigure}
	\hfill
	\begin{subfigure}[t]{0.24\columnwidth}
		\centering
		\input{\fighome/a2c_acktr_app/HalfCheetah_acktr_e=1.0.tex}
	% \caption{VPG on CartPole}
	% \label{sfig:vpg_cart}
	\end{subfigure}
	% \vspace*{-1em}
	\caption{\small{Additional Results for comparison of mean rewards of VPG, PPO, A2C, ACKTR on various environments, with no poisoning, random poisoning, \ourmodtwo and \ourmod. }}
	\label{fig:poison_add}
\end{figure}
% \vspace*{-0.5em}
