# Supplementary material for: Vulnerability-Aware Poisoning Mechanism for Online RL with Unknown Dynamics
Source: arXiv:2009.00774 source file (2022-02-15)
Supplement: Supplementary file 4 [file proof.tex]

%!TEX root = ../0_neurips2020_poisonrl_main.tex

\section{Proofs}
