# Supplementary material for: Vulnerability-Aware Poisoning Mechanism for Online RL with Unknown Dynamics
Source: arXiv:2009.00774 source file (2022-02-15)
Supplement: Supplementary file 5 [file related_works.tex]

%!TEX root = ../0_neurips2020_poisonrl_main.tex
\section{Additional Related Works}
\label{app:relatedworks}

% The security of RL  in some high-stake areas~\citep{zhang2018human,gottesman2019guidelines}. 

\textbf{Adversarial Attacks in Supervised Learning }
Adversarial attacking and defending are attracting more and more attention nowadays~\citep{huang2011adversarial,biggio2012poisoning,steinhardt2017certified}.
Poisoning, as one popular type of adversarial attacking, has been well-studied in the field of machine learning~\citep{biggio2012poisoning,mei2015using}, including deep learning~\citep{munoz2017towards,shafahi2018poison}. \citet{wang2018data} consider online learning, which is similar to ours. However, they focus on supervised learning, where the attacker knows all the data stream, while in our RL setting, the whole training data stream is not available to the attacker (as Challenge I states).

\textbf{Poisoning in Reinforcement Learning}
Some related works focus on poisoning stochastic bandits~\cite{jun2018adversarial,liu2019data} and contextual bandits~\cite{ma2018data}. 
Policy teaching (targeted poisoning) is a specific type of poisoning for RL, where the attacker could lead the agent to learn a pre-defined target policy by manipulating the rewards~\cite{zhang2008value,zhang2009policy} or dynamics~\cite{rakhsha2020policy} of the MDP. However, they require the attackers to have prior knowledge of the environments (e.g., the dynamics of the MDP), which is often unrealistic or difficult in practice. 
\citet{ma2019policy} introduce a policy teaching framework for batch-learning model-based agents, while the attacker knows the MDP and the training data batch before the agent learns.
\citet{huang2019deceptive} propose a reward-poisoning attack model, and provide convergence analysis for Q-learning. However, the introduced attack also requires the attacker has a perfect knowledge of the MDP.
\citet{behzadan2017vulnerability} achieve policy poisoning on DQN by crafting perturbed states such that the target action is selected by the leaner, which is analogous to supervised learning, and the data-correlation problem of RL is not considered.

% \textbf{Adversarial Examples in RL}
\textbf{Evasion Attacks in Reinforcement}
As summarized by~\citet{chen2019adversarial}, evasion attacks at test-time such as adversarial perturbation and defense mechanisms in deep reinforcement learning (DRL) are under rapid development. %attracting more and more researchers. 
A line of works consider adversarial perturbations on observations, similar to adversarial examples in supervised learning. 
\citet{huang2017adversarial} first show that neural network policies are vulnerable to evasion attacks on states, by generating state perturbation with fast gradient sign method (FGSM)~\citep{goodfellow2014explaining}.
\citet{lin2017tactics} consider the data-correlation problem in RL, and propose a strategical attack method, which perturbs an input state $s$ only if the agent has ``a strong preference on action selection'', i.e., $\max_a \pi(a|s) - \min_a \pi(a|s)$ is large. This work and our works both consider the constraint that the attacker is only able to attack for limited times, and provide strategies to decide ``when to attack'' to maximize the attacker's profit. However, our work deals with poisoning attacks, which can not be tackled by the method in \citep{lin2017tactics} since the agent does not follow a good policy with effective ``action preference'' in training time.
% We estimate the vulnerability of the agent and only poison when the agent is vulnerable to poisoning.

In addition, \citet{gleave2019adversarial} show that choosing an adversarial policy in multi-agent RL could also negatively affect the victim agent.
There is also a line of work focusing on adversarial examples in path-finding problems~\cite{xiang2018pca,bai2018adversarial}.
